# Supplementary material for: Intra-domain and cross-domain transfer learning for time series data -- How transferable are the features?
Source: arXiv:2201.04449 source file (2022-01-12)
Supplement: Supplementary file 1 [file supplement.tex]

\documentclass{article}
\usepackage[utf8]{inputenc}

\usepackage{graphicx}
\usepackage{multirow}
\usepackage{fixltx2e}
\usepackage{geometry}
\usepackage{placeins}
\usepackage{float}
\usepackage[table]{xcolor}% http://ctan.org/pkg/xcolor

\definecolor{green}{RGB}{103, 255, 90}
\definecolor{red}{RGB}{255, 90, 90}

% allows for temporary adjustment of side margins
\usepackage{chngpage}

\geometry{
  paperwidth=25cm,
  paperheight=33.8cm,
  top=2cm,
  bottom=0cm,
  left=2cm
}

\usepackage[
    singlelinecheck=false
]{caption}

\begin{document}

\centerline{\huge \textbf{Intra-domain and cross-domain transfer learning for}}
\centerline{\huge \textbf{time series data – How transferable are the features?}}
\vspace{0.5cm}
\centerline{\huge \textbf{Supplementary material}}
\vspace{0.5cm}
\centerline{\Large Otović Erik, Njirjak Marko, Jozinović Dario, Mauša Goran}
\centerline{\Large Michelini Alberto, Štajduhar Ivan}
\vspace{1cm}

%%%
\textbf{\Large Comparison by performance and convergence rate} \\

\parbox{21cm}{Table S1 shows how many times TL models outperformed referent models in intra-domain and cross-domain scenarios. Cross-domain scenario is decomposed into three sub-cases to provide more insight. The models used to obtain Table S1 were also compared by their convergence rate and the results of comparison are shown in Table S2.}

\FloatBarrier
\parbox{21cm}{
    \input{wins_loses_performance}
    \input{wins_loses_convergence}
}
\newpage

%%%
\eject \pdfpagewidth=25cm \pdfpageheight=11.3cm
\textbf{\Large Relationship between performance and convergence rate} \\

\parbox{21cm}{Table S3 shows the relationship between the change in convergence rate and performance score for TL and referent models. In the 140 cases, TL models performed and converged better than referent models. The TL model only performed better than the referent models in 77 cases, while in 13 cases they only converged faster. Only in 10 cases, TL models performed worse and converged slower than referent models.}

\parbox{21cm}{
    \input{relationship_convergence_performance}
}
\newpage

%%%
\eject \pdfpagewidth=25cm \pdfpageheight=17.8cm
\textbf{\Large Influence of model on the transfer learning} \\

\parbox{21cm}{Table S4 shows how many times each TL model outperformed its referent models in intra-domain and cross-domain scenarios.\\ Cross-domain scenario is decomposed into three sub-cases for better perception. This table is obtained in the same way as Table S1. However, the results are shown per model, so  conclusions on the influence of models on  transfer learning can be drawn.}

\parbox{21cm}{
    \input{influence_of_chosen_model}
}
\newpage

%%%
\eject \pdfpagewidth=47.92cm \pdfpageheight=33.7cm
\parbox{21cm}{\textbf{\Large Detailed results for the change in predictive performance and convergence rate}}\\

\parbox{21cm}{
    Tables S5 and S6 show the average difference in predictive performance and converge rate between transfer learning and referent models for each examined triplet (model, source dataset, target dataset). First column contains the pairs of architectures and source datasets that were used for pre-training and were later trained on the target tasks shown in the first row. 

    Each cell contains the average difference for seven reruns of the experiment and the p-value from Wilcoxon signed-rank test is shown in the brackets. Cases in which a statistically significant difference was found by a statistical test (significance level of 0.05) are colored in green and red. Green color indicates that transfer learning models significantly outperformed referent models, while red color indicates that referent models significantly outperformed transfer learning models. Benjamini-Krieger-Yekutieli correction is not applied to this two tables. 
}

\vspace{0.5cm}

%%\parbox{1400pt}{
    \begin{table}[h]
\caption{Average percentual gain in predictive performance across seven reruns of the experiment.}
\begin{adjustwidth}{-1in}{-1in} % adjust the L and R margins by 1 inch
\hspace*{7em}
\begin{tabular}{|l|l|l|l|l|l|l|l|l|l|l|l|l|}
\hline
  & \textbf{LOMAX 1k5} & \textbf{LOMAX 9k} & \textbf{LEN-DB 1k5} & \textbf{LEN-DB 9k} & \textbf{STEAD 1k5} & \textbf{STEAD 9k} & \textbf{SPEECH 1k5} & \textbf{SPEECH 9k} & \textbf{EMG 1k5} & \textbf{EMG 9k} & \textbf{S\&P 500 1k5} & \textbf{S\&P 500 9k}\\ \hline
ConvNetQuake INGV [LOMAX] & - & - & \cellcolor{green} 13.6\% (0.01796) & 0.226\% (0.7353) & \cellcolor{green} 5.63\% (0.01796) & \cellcolor{green} 3.16\% (0.01796) & \cellcolor{red} -29.6\% (0.02799) & \cellcolor{green} 7.95e+02\% (0.01796) & \cellcolor{green} 29.3\% (0.02799) & \cellcolor{green} 40.2\% (0.01796) & \cellcolor{green} 80.8\% (0.01796) & \cellcolor{green} 77.1\% (0.01796) \\ \hline
MagNet [LOMAX] & - & - & 2.59\% (0.2367) & 0.7\% (1.0) & 5.68\% (0.09097) & 4.31\% (0.3105) & \cellcolor{green} 28.1\% (0.04252) & \cellcolor{green} 1.62e+03\% (0.01796) & \cellcolor{green} 26.0\% (0.02799) & \cellcolor{green} 10.7\% (0.01796) & \cellcolor{green} 2.04\% (0.01796) & \cellcolor{green} 2.07\% (0.02799) \\ \hline
MLSTM FCN [LOMAX] & - & - & \cellcolor{green} 2.88\% (0.01796) & 1.24\% (0.3105) & \cellcolor{green} 5.65\% (0.01796) & \cellcolor{green} 1.36\% (0.01796) & \cellcolor{green} 81.3\% (0.01796) & 4.88\% (0.09097) & \cellcolor{green} 19.6\% (0.01796) & \cellcolor{green} 5.54\% (0.01796) & \cellcolor{green} 75.6\% (0.01796) & \cellcolor{green} 9.33\% (0.02799) \\ \hline
TCN [LOMAX] & - & - & \cellcolor{green} 13.7\% (0.02799) & \cellcolor{green} 10.5\% (0.01796) & \cellcolor{green} 9.58\% (0.02799) & \cellcolor{green} 7.03\% (0.01796) & \cellcolor{green} 1.03e+02\% (0.01796) & \cellcolor{green} 1.06e+03\% (0.01796) & \cellcolor{green} 21.8\% (0.01796) & \cellcolor{green} 13.8\% (0.01796) & \cellcolor{green} 23.2\% (0.01796) & \cellcolor{green} 2.75\% (0.01796) \\ \hline
ConvNetQuake INGV [LEN-DB] & 2.86\% (0.499) & 2.44\% (0.7353) & - & - & \cellcolor{green} 6.38\% (0.04252) & 0.684\% (0.1282) & \cellcolor{green} 7.62e+02\% (0.01796) & \cellcolor{green} 1.76e+03\% (0.01796) & \cellcolor{green} 25.0\% (0.02799) & \cellcolor{green} 29.5\% (0.02799) & \cellcolor{green} 81.2\% (0.01796) & \cellcolor{green} 76.5\% (0.01796) \\ \hline
MagNet [LEN-DB] & \cellcolor{green} 6.61\% (0.01796) & \cellcolor{green} 6.98\% (0.01796) & - & - & 3.07\% (0.09097) & \cellcolor{green} 2.1\% (0.01796) & \cellcolor{green} 2.75e+02\% (0.01796) & \cellcolor{green} 2.12e+03\% (0.01796) & \cellcolor{green} 28.7\% (0.02799) & \cellcolor{green} 12.5\% (0.01796) & 1.41\% (0.06298) & \cellcolor{green} 1.28\% (0.04252) \\ \hline
MLSTM FCN [LEN-DB] & \cellcolor{green} 7.19\% (0.01796) & \cellcolor{green} 2.55\% (0.01796) & - & - & \cellcolor{green} 5.69\% (0.01796) & \cellcolor{green} 0.863\% (0.04252) & \cellcolor{green} 67.2\% (0.01796) & -0.984\% (0.6121) & \cellcolor{green} 16.3\% (0.01796) & -0.759\% (0.499) & \cellcolor{green} 73.8\% (0.01796) & \cellcolor{green} 8.4\% (0.01796) \\ \hline
TCN [LEN-DB] & 16.3\% (0.06298) & 4.08\% (0.1763) & - & - & -5.18\% (0.06298) & \cellcolor{green} 6.42\% (0.01796) & \cellcolor{green} 1.32e+02\% (0.01796) & \cellcolor{green} 9.63e+02\% (0.01796) & \cellcolor{green} 17.7\% (0.01796) & \cellcolor{green} 7.4\% (0.01796) & \cellcolor{green} 21.2\% (0.01796) & 2.1\% (0.06298) \\ \hline
ConvNetQuake INGV [STEAD] & -20.0\% (0.1763) & -10.9\% (0.398) & -0.601\% (0.7353) & -8.65\% (0.2367) & - & - & \cellcolor{green} 8.59e+02\% (0.01796) & \cellcolor{green} 1.7e+03\% (0.01796) & \cellcolor{green} 25.5\% (0.01796) & \cellcolor{green} 29.5\% (0.02799) & \cellcolor{green} 81.7\% (0.01796) & \cellcolor{green} 76.4\% (0.01796) \\ \hline
MagNet [STEAD] & \cellcolor{green} 6.62\% (0.01796) & \cellcolor{green} 5.59\% (0.01796) & -0.112\% (0.8658) & 0.187\% (0.6121) & - & - & \cellcolor{green} 3.11e+02\% (0.01796) & \cellcolor{green} 2.12e+03\% (0.01796) & \cellcolor{green} 28.3\% (0.02799) & \cellcolor{green} 14.2\% (0.01796) & 1.35\% (0.06298) & \cellcolor{green} 1.63\% (0.04252) \\ \hline
MLSTM FCN [STEAD] & \cellcolor{green} 7.13\% (0.01796) & 1.75\% (0.09097) & \cellcolor{green} 3.09\% (0.01796) & -0.296\% (0.6121) & - & - & \cellcolor{green} 60.7\% (0.01796) & -2.75\% (0.09097) & \cellcolor{green} 13.9\% (0.01796) & -2.01\% (0.2367) & \cellcolor{green} 74.7\% (0.01796) & \cellcolor{green} 10.2\% (0.01796) \\ \hline
TCN [STEAD] & 10.9\% (0.09097) & -3.95\% (0.499) & -0.152\% (1.0) & \cellcolor{green} 6.7\% (0.01796) & - & - & \cellcolor{green} 61.6\% (0.01796) & \cellcolor{green} 5.05e+02\% (0.01796) & 7.01\% (0.06298) & -1.44\% (0.398) & \cellcolor{green} 19.6\% (0.01796) & \cellcolor{green} 2.39\% (0.01796) \\ \hline
ConvNetQuake INGV [SPEECH] & \cellcolor{green} 5.66\% (0.04252) & \cellcolor{green} 10.1\% (0.01796) & \cellcolor{green} 10.5\% (0.02799) & \cellcolor{green} 2.32\% (0.01796) & \cellcolor{red} -6.52\% (0.02799) & \cellcolor{green} 2.98\% (0.02799) & - & - & \cellcolor{green} 33.5\% (0.01796) & \cellcolor{green} 48.2\% (0.01796) & \cellcolor{green} 79.8\% (0.01796) & \cellcolor{green} 74.2\% (0.01796) \\ \hline
MagNet [SPEECH] & -1.09\% (0.7353) & 3.45\% (0.09097) & 0.919\% (0.7353) & -0.37\% (0.398) & -0.0623\% (1.0) & 0.575\% (0.8658) & - & - & \cellcolor{green} 6.91\% (0.02799) & -1.91\% (0.3105) & \cellcolor{green} 1.66\% (0.01796) & 1.0\% (0.2367) \\ \hline
MLSTM FCN [SPEECH] & \cellcolor{green} 5.14\% (0.02799) & 0.612\% (0.7353) & \cellcolor{green} 2.83\% (0.01796) & 0.481\% (0.7353) & -0.782\% (0.499) & -1.69\% (0.2367) & - & - & 3.76\% (0.3105) & -2.79\% (0.398) & \cellcolor{green} 74.5\% (0.01796) & \cellcolor{green} 9.58\% (0.01796) \\ \hline
TCN [SPEECH] & \cellcolor{green} 27.4\% (0.01796) & 0.202\% (0.499) & \cellcolor{green} 3.63\% (0.02799) & \cellcolor{green} 10.3\% (0.01796) & -1.86\% (0.2367) & -1.58\% (0.7353) & - & - & \cellcolor{green} 9.81\% (0.01796) & -3.97\% (0.06298) & \cellcolor{green} 20.3\% (0.01796) & \cellcolor{green} 1.5\% (0.04252) \\ \hline
ConvNetQuake INGV [EMG] & \cellcolor{green} 4.92\% (0.02799) & \cellcolor{green} 14.2\% (0.01796) & \cellcolor{green} 6.64\% (0.02799) & \cellcolor{green} 1.98\% (0.01796) & -2.1\% (0.398) & \cellcolor{green} 3.17\% (0.02799) & \cellcolor{green} 1.18e+03\% (0.01796) & \cellcolor{green} 4.07e+03\% (0.01796) & - & - & \cellcolor{green} 76.1\% (0.01796) & \cellcolor{green} 72.0\% (0.01796) \\ \hline
MagNet [EMG] & \cellcolor{green} 4.11\% (0.01796) & 1.71\% (0.398) & -2.29\% (0.3105) & -0.706\% (0.2367) & 2.84\% (0.3105) & \cellcolor{green} 2.2\% (0.02799) & \cellcolor{green} 1.04e+02\% (0.01796) & \cellcolor{green} 2.16e+03\% (0.01796) & - & - & 0.967\% (0.1282) & 0.92\% (0.3105) \\ \hline
MLSTM FCN [EMG] & \cellcolor{green} 6.69\% (0.01796) & \cellcolor{green} 2.33\% (0.01796) & \cellcolor{green} 2.86\% (0.01796) & \cellcolor{green} 1.92\% (0.04252) & \cellcolor{green} 6.29\% (0.01796) & \cellcolor{green} 1.51\% (0.01796) & \cellcolor{green} 89.5\% (0.01796) & \cellcolor{green} 6.55\% (0.04252) & - & - & \cellcolor{green} 69.2\% (0.01796) & -2.45\% (0.8658) \\ \hline
TCN [EMG] & \cellcolor{green} 20.8\% (0.01796) & 3.12\% (0.3105) & \cellcolor{red} -7.43\% (0.01796) & -1.57\% (0.499) & -2.44\% (0.06298) & 1.29\% (0.398) & \cellcolor{green} 96.6\% (0.01796) & \cellcolor{green} 1.04e+03\% (0.01796) & - & - & \cellcolor{green} 21.1\% (0.01796) & \cellcolor{green} 2.42\% (0.01796) \\ \hline
ConvNetQuake INGV [S\&P 500] & -14.0\% (0.2367) & 0.439\% (1.0) & 1.58\% (0.7353) & 1.37\% (0.2367) & -20.0\% (0.2367) & -5.24\% (0.2367) & \cellcolor{green} 2.61e+02\% (0.01796) & \cellcolor{green} 1.01e+03\% (0.01796) & \cellcolor{green} 34.1\% (0.01796) & \cellcolor{green} 39.8\% (0.01796) & - & - \\ \hline
MagNet [S\&P 500] & -8.96\% (0.1282) & -2.51\% (0.499) & -7.98\% (0.06298) & -0.912\% (0.2367) & 1.04\% (0.6121) & 0.504\% (0.8658) & \cellcolor{green} 65.7\% (0.02799) & \cellcolor{green} 1.75e+03\% (0.01796) & \cellcolor{green} 8.71\% (0.02799) & \cellcolor{green} 7.61\% (0.01796) & - & - \\ \hline
MLSTM FCN [S\&P 500] & \cellcolor{green} 3.61\% (0.04252) & 0.165\% (0.7353) & 1.49\% (0.1282) & 0.266\% (0.8658) & -2.13\% (0.2367) & -0.874\% (0.2367) & \cellcolor{green} 1.01e+02\% (0.01796) & \cellcolor{green} 9.84\% (0.01796) & 4.69\% (0.2367) & 0.467\% (0.8658) & - & - \\ \hline
TCN [S\&P 500] & \cellcolor{green} 19.8\% (0.04252) & 2.33\% (0.2367) & 1.22\% (0.1763) & \cellcolor{green} 3.81\% (0.04252) & \cellcolor{red} -7.88\% (0.04252) & -3.54\% (0.2367) & \cellcolor{green} 59.0\% (0.01796) & \cellcolor{green} 7.64e+02\% (0.01796) & \cellcolor{green} 13.1\% (0.01796) & -0.348\% (1.0) & - & - \\ \hline
\end{tabular}
\end{adjustwidth}
\end{table}

\begin{table}[h]
\caption{Average percentual gain in convergence rate across seven reruns of the experiment for the hyperparameters that achieved the best predictive performance.}
\begin{adjustwidth}{-1in}{-1in} % adjust the L and R margins by 1 inch
\hspace*{7em}
\begin{tabular}{|l|l|l|l|l|l|l|l|l|l|l|l|l|}
\hline
  & \textbf{LOMAX 1k5} & \textbf{LOMAX 9k} & \textbf{LEN-DB 1k5} & \textbf{LEN-DB 9k} & \textbf{STEAD 1k5} & \textbf{STEAD 9k} & \textbf{SPEECH 1k5} & \textbf{SPEECH 9k} & \textbf{EMG 1k5} & \textbf{EMG 9k} & \textbf{S\&P 500 1k5} & \textbf{S\&P 500 9k}\\ \hline
ConvNetQuake INGV [LOMAX] & - & - & 9.61\%  (0.09097) & -7.56\%  (0.1763) & \cellcolor{green} 14.1\% (0.02799) & -1.92\%  (0.499) & -12.2\%  (0.1763) & -14.0\%  (0.06298) & 16.0\%  (0.06298) & 0.501\%  (0.6121) & \cellcolor{green} 5.3\% (0.02799) & 14.8\%  (0.1763) \\ \hline
MagNet [LOMAX] & - & - & 43.5\%  (0.2367) & -9.19\%  (0.499) & 32.6\%  (0.398) & 41.6\%  (0.1282) & 13.2\%  (0.1763) & -8.05\%  (0.499) & 12.3\%  (0.1282) & -0.491\%  (1.0) & \cellcolor{green} 5.35\% (0.01796) & \cellcolor{green} 3.06\% (0.01796) \\ \hline
MLSTM FCN [LOMAX] & - & - & \cellcolor{red} -5.98\% (0.01796) & -1.71\%  (0.6121) & -8.85\%  (0.1282) & 1.63\%  (0.8658) & 3.47\%  (0.2367) & \cellcolor{green} 5.94\% (0.01796) & 3.47\%  (0.398) & \cellcolor{red} -13.8\% (0.01796) & \cellcolor{green} 13.2\% (0.01796) & 1.4\%  (0.1763) \\ \hline
TCN [LOMAX] & - & - & -10.8\%  (0.1282) & 5.87\%  (0.2367) & 28.6\%  (0.09097) & 5.27\%  (0.6121) & -3.96\%  (0.2367) & \cellcolor{green} 34.4\% (0.01796) & \cellcolor{green} 21.3\% (0.02799) & 6.21\%  (0.06298) & 1.62\%  (0.8658) & 2.25\%  (0.2367) \\ \hline
ConvNetQuake INGV [LEN-DB] & 30.2\%  (0.06298) & 13.7\%  (0.2367) & - & - & 32.4\%  (0.2367) & -6.31\%  (1.0) & \cellcolor{green} 14.0\% (0.02799) & -4.24\%  (0.398) & -1.95\%  (0.6121) & -0.459\%  (0.8658) & \cellcolor{green} 3.8\% (0.01796) & 9.19\%  (0.7353) \\ \hline
MagNet [LEN-DB] & \cellcolor{green} 7.72\% (0.02799) & -0.0567\%  (0.398) & - & - & 0.901\%  (0.3105) & 21.6\%  (0.6121) & -1.33\%  (0.7353) & 6.05\%  (0.09097) & \cellcolor{green} 17.0\% (0.01796) & -5.45\%  (0.06298) & \cellcolor{green} 5.63\% (0.01796) & \cellcolor{green} 3.49\% (0.02799) \\ \hline
MLSTM FCN [LEN-DB] & 0.278\%  (0.499) & -3.84\%  (0.1282) & - & - & 5.71\%  (0.3105) & 3.38\%  (0.2367) & 5.65\%  (0.2367) & 4.76\%  (0.06298) & \cellcolor{green} 11.9\% (0.02799) & \cellcolor{red} -13.9\% (0.02799) & \cellcolor{green} 13.0\% (0.04252) & \cellcolor{green} 1.92\% (0.04252) \\ \hline
TCN [LEN-DB] & \cellcolor{green} 8.38\% (0.01796) & 17.1\%  (0.7353) & - & - & \cellcolor{green} 30.8\% (0.01796) & \cellcolor{green} 28.4\% (0.04252) & \cellcolor{red} -13.8\% (0.01796) & \cellcolor{green} 24.9\% (0.01796) & \cellcolor{green} 41.1\% (0.01796) & 5.18\%  (0.3105) & 3.3\%  (0.1282) & 0.0614\%  (0.7353) \\ \hline
ConvNetQuake INGV [STEAD] & 28.2\%  (0.3105) & 15.0\%  (0.09097) & \cellcolor{green} 57.4\% (0.01796) & 10.2\%  (0.6121) & - & - & \cellcolor{green} 17.1\% (0.01796) & 3.98\%  (1.0) & 2.91\%  (0.7353) & -9.11\%  (0.1282) & \cellcolor{green} 5.2\% (0.01796) & 30.3\%  (0.06298) \\ \hline
MagNet [STEAD] & \cellcolor{green} 26.4\% (0.01796) & -8.91\%  (0.1763) & 8.93\%  (0.499) & -4.69\%  (0.2367) & - & - & -11.9\%  (0.09097) & 2.33\%  (0.8658) & \cellcolor{green} 14.7\% (0.02799) & -5.3\%  (0.1282) & \cellcolor{green} 4.51\% (0.02799) & 2.15\%  (0.09097) \\ \hline
MLSTM FCN [STEAD] & -0.323\%  (0.8658) & -6.57\%  (0.06298) & -2.22\%  (0.398) & \cellcolor{red} -10.3\% (0.01796) & - & - & 5.28\%  (0.3105) & 1.98\%  (0.398) & \cellcolor{green} 17.9\% (0.02799) & \cellcolor{red} -18.1\% (0.01796) & \cellcolor{green} 12.6\% (0.02799) & \cellcolor{green} 1.92\% (0.01796) \\ \hline
TCN [STEAD] & \cellcolor{green} 11.9\% (0.01796) & 18.9\%  (0.7353) & \cellcolor{green} 26.3\% (0.01796) & \cellcolor{green} 35.1\% (0.01796) & - & - & -1.0\%  (0.8658) & 5.32\%  (0.3105) & \cellcolor{green} 33.6\% (0.01796) & 3.73\%  (0.3105) & \cellcolor{green} 2.32\% (0.04252) & \cellcolor{green} 4.46\% (0.02799) \\ \hline
ConvNetQuake INGV [SPEECH] & 18.7\%  (0.499) & 8.69\%  (0.7353) & 27.9\%  (0.8658) & 0.346\%  (0.3105) & 1.72\%  (0.1763) & \cellcolor{red} -6.38\% (0.04252) & - & - & \cellcolor{green} 16.6\% (0.02799) & 6.86\%  (0.6121) & \cellcolor{green} 2.93\% (0.02799) & 4.4\%  (1.0) \\ \hline
MagNet [SPEECH] & \cellcolor{green} 21.0\% (0.01796) & \cellcolor{red} -9.98\% (0.02799) & \cellcolor{red} -11.5\% (0.01796) & -2.2\%  (0.7353) & 4.7\%  (0.1763) & 2.55\%  (0.499) & - & - & 11.8\%  (0.06298) & \cellcolor{red} -5.93\% (0.04252) & \cellcolor{green} 5.75\% (0.01796) & \cellcolor{green} 2.61\% (0.01796) \\ \hline
MLSTM FCN [SPEECH] & -4.94\%  (0.1282) & -6.29\%  (0.2367) & -2.66\%  (0.1763) & \cellcolor{red} -8.39\% (0.01796) & \cellcolor{red} -5.73\% (0.01796) & 16.3\%  (0.8658) & - & - & 3.04\%  (0.8658) & \cellcolor{red} -15.7\% (0.02799) & \cellcolor{green} 14.2\% (0.01796) & \cellcolor{green} 1.46\% (0.04252) \\ \hline
TCN [SPEECH] & \cellcolor{green} 5.91\% (0.04252) & 20.3\%  (0.6121) & 8.03\%  (0.398) & 15.6\%  (0.2367) & 26.2\%  (0.1763) & 22.4\%  (0.398) & - & - & 24.0\%  (0.1763) & -5.66\%  (0.6121) & 1.63\%  (0.6121) & \cellcolor{green} 4.07\% (0.01796) \\ \hline
ConvNetQuake INGV [EMG] & 19.9\%  (0.7353) & 14.6\%  (0.06298) & 25.5\%  (0.2367) & -5.41\%  (0.3105) & \cellcolor{green} 28.3\% (0.01796) & 0.0097\%  (0.398) & 26.5\%  (0.1282) & 2.38\%  (0.499) & - & - & \cellcolor{green} 3.56\% (0.01796) & 26.5\%  (0.2367) \\ \hline
MagNet [EMG] & \cellcolor{green} 16.1\% (0.01796) & -13.1\%  (0.09097) & 21.0\%  (0.6121) & -2.71\%  (0.8658) & 15.9\%  (0.06298) & 37.3\%  (0.09097) & 4.45\%  (0.3105) & 6.91\%  (0.1282) & - & - & \cellcolor{green} 3.67\% (0.01796) & 2.18\%  (0.06298) \\ \hline
MLSTM FCN [EMG] & 1.11\%  (0.398) & -0.467\%  (0.8658) & -2.33\%  (0.06298) & \cellcolor{red} -8.68\% (0.04252) & \cellcolor{red} -6.81\% (0.01796) & \cellcolor{green} 9.81\% (0.04252) & 5.39\%  (0.3105) & 3.09\%  (0.1282) & - & - & \cellcolor{green} 13.7\% (0.01796) & 0.515\%  (0.2367) \\ \hline
TCN [EMG] & 3.45\%  (0.3105) & 22.1\%  (0.1282) & 15.2\%  (0.8658) & 15.6\%  (0.7353) & -1.47\%  (0.7353) & 4.17\%  (0.7353) & \cellcolor{red} -13.3\% (0.01796) & \cellcolor{green} 25.0\% (0.01796) & - & - & \cellcolor{green} 3.89\% (0.04252) & \cellcolor{green} 3.78\% (0.02799) \\ \hline
ConvNetQuake INGV [S\&P 500] & 12.0\%  (0.2367) & 13.6\%  (0.09097) & 35.0\%  (0.499) & 6.22\%  (0.8658) & 32.5\%  (0.2367) & 19.0\%  (0.2367) & 7.4\%  (0.3105) & -4.75\%  (0.398) & 1.62\%  (0.6121) & -0.0643\%  (0.8658) & - & - \\ \hline
MagNet [S\&P 500] & -2.88\%  (0.3105) & -8.59\%  (0.398) & 20.6\%  (0.398) & -8.83\%  (0.499) & 13.6\%  (0.2367) & 6.05\%  (0.1282) & 8.78\%  (0.1763) & 1.23\%  (0.8658) & 6.56\%  (0.499) & -4.52\%  (0.3105) & - & - \\ \hline
MLSTM FCN [S\&P 500] & -0.267\%  (0.3105) & -5.95\%  (0.1763) & -3.92\%  (0.09097) & \cellcolor{red} -8.61\% (0.01796) & \cellcolor{red} -5.88\% (0.04252) & 8.91\%  (0.3105) & 7.4\%  (0.2367) & 4.08\%  (0.3105) & 2.79\%  (0.398) & \cellcolor{red} -15.9\% (0.02799) & - & - \\ \hline
TCN [S\&P 500] & \cellcolor{green} 7.34\% (0.01796) & 18.2\%  (0.7353) & 3.44\%  (1.0) & 5.64\%  (0.2367) & -1.19\%  (0.398) & 21.6\%  (0.6121) & -4.4\%  (0.6121) & \cellcolor{green} 22.4\% (0.02799) & 21.5\%  (0.1282) & -3.84\%  (0.398) & - & - \\ \hline
\end{tabular}
\end{adjustwidth}
\end{table}
%%}
\end{document}
